# Supplementary material for: Risk mapping for COVID-19 outbreaks in Australia using mobility data
Source: arXiv:2008.06193 ancillary file (2020-12-04)
Supplement: Supplementary file 1 [file Supplementary_Technical_Note.pdf]

# Technical note: interpolation of Origin-Destination mobility data between different geospatial partition schemes

Cameron Zachreson<sup>1</sup>

<sup>1</sup>*The University of Melbourne, Melbourne School of Engineering,  
School of Computing and Information Systems*

## Abstract

Origin-destination matrices that represent the movement of populations between regions are ubiquitous data structures used frequently when building models of infectious disease transmission in mobile populations. Of course, the topology of such matrices depends on the classifications used to define regions (nodes) of the matrix. Typically the nodes of an origin-destination matrix are defined spatial regions, but any unique set of classifiers may be used to describe the flows of individuals between compartments. Often, it is necessary to interpolate data from one set of classifiers (regions) into a different, possibly overlapping, set. In this note, I describe a simple method and algorithm for performing this type of interpolation using correspondences represented as conditional probabilities of regional occupancy.

## I. OVERVIEW

Given:

- set of  $N$  origins ( $O$ ), these could be spatial regions, or any other appropriate classifier
- set of  $M$  destinations ( $D$ ), this can be the same set of partitions used for origins, or it can be some other set of classifiers
- An  $N \times M$  asymmetric, weighted adjacency matrix ( $\mathbf{G}$ ), in which each element  $G_{ij}$  describes the movement of discrete quantities (i.e., populations) from origin node  $i \in [1, N]$  to destination node  $j \in [1, M]$
- set of  $L$  partitions ( $O^*$ ) that will be the set of origins after re-partitioning
- set of  $K$  partitions ( $D^*$ ) that will be the set of destinations after re-partitioning
- A correspondence  $O \rightarrow O^*$ . For example, a  $N \times L$  matrix  $\mathbf{P}_O$  of conditional probabilities  $p_{nk}(O_k^* | O_n)$  describing the probability that an individual will be found in the  $k$ -th region of the set  $O^*$  given that they are in the  $n$ -th region of the set  $O$ .
- A correspondence  $D \rightarrow D^*$ , e.g., a  $M \times K$  matrix  $\mathbf{P}_D$  of conditional probabilities describing the correspondence between destinations (see above).

The method uses the correspondences  $\mathbf{P}_D$  and  $\mathbf{P}_O$  to re-partition the elements of  $\mathbf{G}$  into a new  $L \times K$  matrix  $\mathbf{G}^*$ .

## II. METHODS

Once the partition sets and their correspondences are in hand, the method is straightforward and proceeds as per the example illustrated in Figure 1. Each connection between the new sets of partitions consists of a linear combination of components, one for each edge in the original matrix  $\mathbf{G}$ . For origin  $A$  and destination  $B$  in the original matrix  $\mathbf{G}$ , let  $G(A \rightarrow B)$  represent the flow of individuals from  $A$  to  $B$ . For origin  $x$  and destination  $y$  in the new matrix  $\mathbf{G}^*$ , the contribution of  $G(A \rightarrow B)$  is computed as follows:

$$G^*(x \rightarrow y) = \sum_{i, j} G(A_i \rightarrow B_j) \times P_O(A_i, x) \times P_D(B_j, y) \quad (1)$$

in which subscripts  $i, j$  indicate summation over all elements of  $\mathbf{G}$  and  $P_O(A, x) = p(x \mid A)$  and  $P_D(B, y) = p(y \mid B)$  are the correspondences between origin and destination regions computed as conditional probabilities. The product  $[P_O(A, x) \times P_D(B, y)]$  gives the probability that an individual departing from region  $A$  and arriving in region  $B$  also departed from region  $x$  to arrive in region  $y$ . Iterating over all pairs  $G(A_i \rightarrow B_j)$  gives the set of factors composing each new connection. Of course, all elements for which  $G(A_i \rightarrow B_j) = 0$ ,  $P_O(A_i, x) = 0$ , or  $P_D(B_j, y) = 0$  may be omitted from the sum in implementation. In the MATLAB implementation included below, these exclusions are implemented implicitly in the sparse input tables, in which zero-valued entries are not included.

By expressing the correspondences  $\mathbf{P}_O$  and  $\mathbf{P}_D$  as  $N \times L$  and  $M \times K$  matrices, respectively, the transformation  $\mathbf{G} \rightarrow \mathbf{G}^*$ , can be succinctly expressed as:

$$\mathbf{G}^* = \mathbf{P}_O^\top \mathbf{G} \mathbf{P}_D \quad (2)$$

While the method presented here is simple to implement, the production of the correspondences  $\mathbf{P}_O$  and  $\mathbf{P}_D$  can be non-trivial and will depend on the type of data represented in the matrix  $\mathbf{G}$ , as well as the types of compartments used for  $O$ ,  $D$ ,  $O^*$ , and  $D^*$ . As an example, consider the common case where  $O^*$  is a particular set of spatial partitions (e.g., administrative regions) and  $O$  is a dramatically different set of regions (e.g., Bing Tiles). To generate a correspondence, it is necessary to establish some type of overlap measure between these regions, this could be spatial, or it could be based on some other quantity that may vary in space (e.g., population), so that spatial overlap can be translated into the desired conditional occupancy probabilities. In the latter case, a useful technique is to find some set of partitions of much smaller scale, so that the quantities of interest (numbers of people, addresses, businesses, etc.) can be over-sampled for each region and the degree of overlap quantified, without requiring data on the level of individual people (which is typically not available).

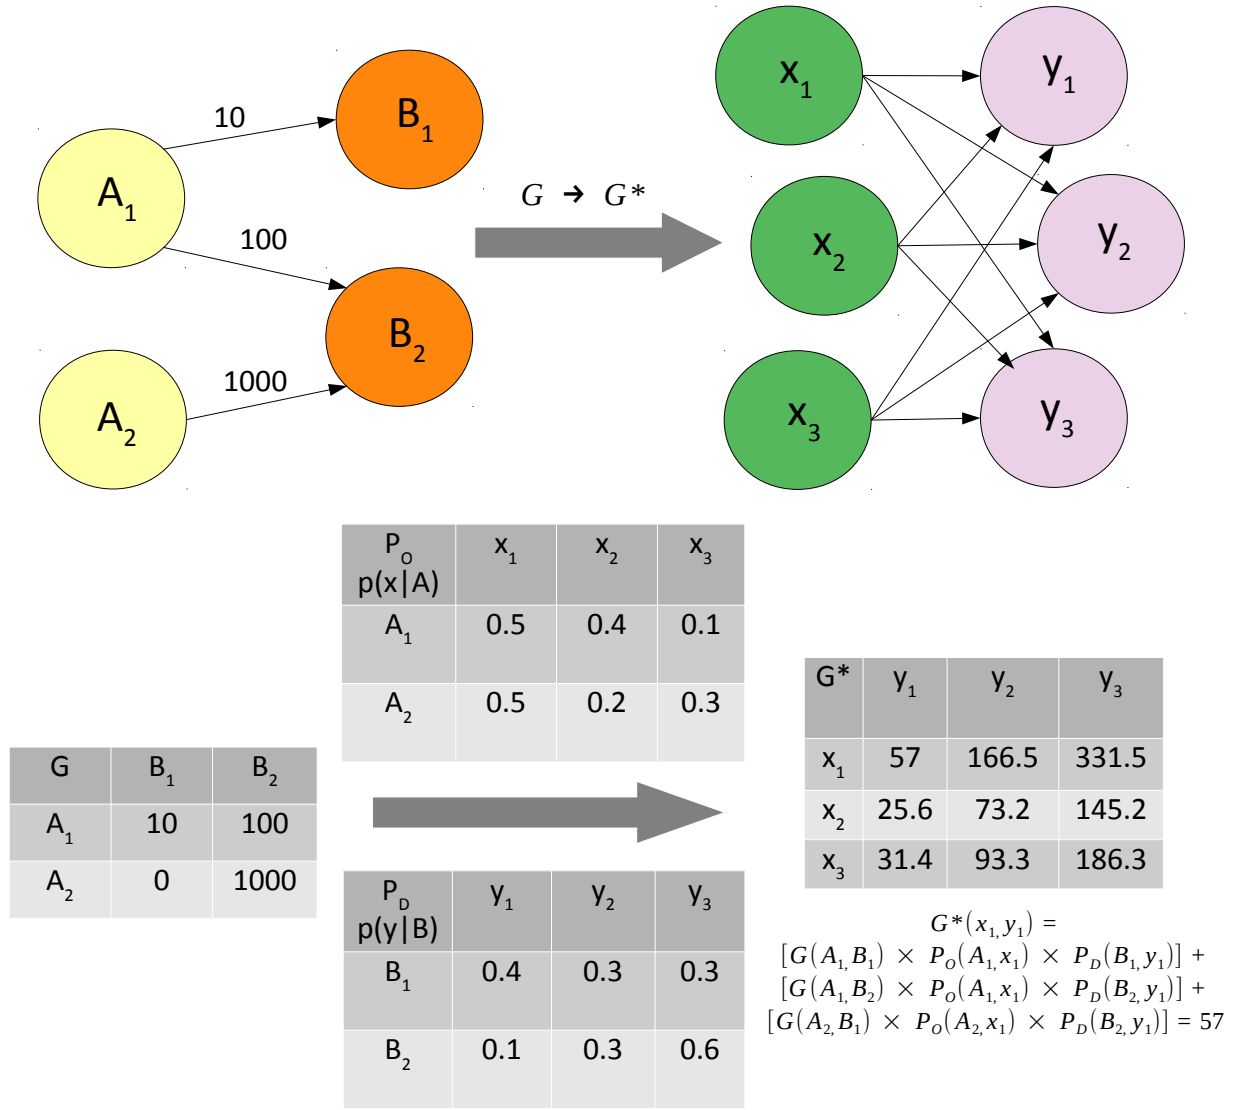

FIG. 1. Schematic of the described procedure

### III. MATLAB IMPLEMENTATION

This code implements the example shown in Figure 1

```
1 % converts a matrix between partition schemes, ingredients are the
2 % original edge list and a correspondence file for conversion of boundaries
3 % between sets.
4
5 % input data structures
6
7 %input files are:
8
9 % OD_test.csv
10 % origin      destination      n
11 % A1          B1                10
12 % A1          B2                100
13 % A2          B2                1000
14
15 % PD.csv
16 % D_old      D_new      p
17 % B1         y1         0.4
18 % B1         y2         0.3
19 % B1         y3         0.3
20 % B2         y1         0.1
21 % B2         y2         0.3
22 % B2         y3         0.6
23
24 % PO.csv
25 % O_old      O_new      p
26 % A1         x1         0.5
27 % A1         x2         0.4
28 % A1         x3         0.1
29 % A2         x1         0.5
30 % A2         x2         0.2
31 % A2         x3         0.3
32
33 % original matrix, to be converted to new partition
34 % scheme -> table columns: {origin, destination, n}
35
36 input_filename = 'OD_test.csv';
37 output_filename = 'OD_out.csv';
38
39 % set up correspondence structures
40
```

```

41 % PO.csv -> table columns: {O_old, O_new, p}
42 % PD.csv -> table columns: {D_old, D_new, p}
43
44 PO_filename = 'PO.csv';
45 PD_filename = 'PD.csv';
46
47 PO_corr_table = readtable(PO_filename);
48 PD_corr_table = readtable(PD_filename);
49
50 orig_IDs = cellstr([ PO_corr_table.O_old ; PD_corr_table.D_old]);
51 new_IDs = cellstr([ PO_corr_table.O_new ; PD_corr_table.D_new]);
52 corr_vals = [PO_corr_table.p ; PD_corr_table.p];
53
54 corr_table = table(orig_IDs, new_IDs, corr_vals);
55
56 orig_ID_list = unique(corr_table.orig_IDs, 'rows');
57
58 % converting correspondence table into map of maps:
59 % outer key values will be old codes
60 % inner key values will be new codes
61 % inner values are the associated correspondence proportion
62
63 corr_map = containers.Map('KeyType', 'char', 'ValueType', 'any');
64
65 % initialise correspondence structure
66 for i = 1:size(orig_ID_list, 1)
67
68     corr_map(orig_ID_list{i}) = containers.Map('KeyType', 'char', ...
69         'ValueType', 'any');
70
71 end
72
73 % fill the inner maps
74 for i = 1:size(corr_table.orig_IDs, 1)
75
76     id_source = corr_table.orig_IDs{i};
77     tmp = corr_map(id_source);
78     id_target = corr_table.new_IDs{i};
79     corr_val = corr_table.corr_vals(i);
80     tmp(id_target) = corr_val;
81     corr_map(id_source) = tmp;
82
83 end
84
85 orig_edges = {};

```

```

86
87 e_table = readtable(input_filename);
88
89 for i = 1:size(e_table, 1)
90     orig_edges{i, 1} = {e_table.origin{i}, e_table.destination{i}, ...
91         double(e_table.n(i))};
92 end
93 % make the new edge list, each edge in the old list will map to edges ...
94 % in the
95 % new list based on the correspondence map.
96 new_edges = containers.Map('KeyType', 'char', 'ValueType', 'any');
97
98 % iterate through the old edge list, and distribute the commuters into the
99 % new edge list
100
101 % imperfect correspondence can lead to lost travellers,
102 % let's count them and see if it's a significant issue:
103 lost_travellers = 0;
104 total_travellers = sum(e_table.n);
105
106 for i = 1:size(orig_edges, 1)
107
108     % each edge will produce a set of source and target nodes based on the
109     % correspondence between partition schemes, these are the key ...
110     % values from
111     % the inner corr_map associated with source and target codes
112
113     old_source = orig_edges{i}{1};
114     old_target = orig_edges{i}{2};
115     w_old = orig_edges{i}{3};
116
117     if ~isKey(corr_map, old_source)
118         lost_travellers = lost_travellers + w_old;
119         fraction_lost = lost_travellers / total_travellers;
120         fprintf(['no correspondence for tile ' old_source ', ', ...
121             '\n fraction travellers lost: ' num2str(fraction_lost) '\n'])
122
123         continue
124     end
125
126     new_source_IDs = keys(corr_map(old_source));
127     corr_source_old = corr_map(old_source);
128

```

```

129     if ~isKey(corr_map, old_target)
130         lost_travellers = lost_travellers + w_old;
131         fraction_lost = lost_travellers / total_travellers;
132         fprintf(['no correspondence for tile ' old_target ' ', ...
133             '\n fraction travellers lost: ' num2str(fraction_lost) '\n'])
134
135         continue
136
137     end
138
139     new_target_IDs = keys(corr_map(old_target));
140     corr_target_old = corr_map(old_target);
141
142     for j = 1:size(new_source_IDs, 2)
143
144         if ~isKey(new_edges, new_source_IDs{j})
145
146             new_edges(new_source_IDs{j}) = ...
147                 containers.Map('KeyType', 'char', 'ValueType', 'any');
148         end
149
150         new_source_id = new_source_IDs{j};
151         proportion_source = corr_source_old(new_source_id);
152         tmp = new_edges(new_source_IDs{j}); %inner map
153
154         for k = 1:size(new_target_IDs, 2)
155
156             new_target_id = new_target_IDs{k};
157             proportion_target = corr_target_old(new_target_id);
158             w_new = w_old * proportion_source * proportion_target;
159
160             %         disp([old_source, ' ', ' ', old_target, ' ', ' ' num2str(w_old) ])
161             %         disp(['p_source: ' num2str(proportion_source), '; ...
162             p_target: '...
163             %             num2str(proportion_target)])
164             %         disp([new_source_id ' ', ' ' new_target_id ' ', ' ...
165             num2str(w_new)])
166             %         disp(' ')
167
168             if ~isKey(tmp, new_target_IDs{k})
169
170                 tmp(new_target_IDs{k}) = w_new;
171
172             else
173
174                 tmp(new_target_IDs{k}) = tmp(new_target_IDs{k}) + w_new;

```

```

173
174         end
175     end
176
177     % update edge map
178     new_edges(new_source_IDs{j}) = tmp;
179
180     end
181 end
182
183 % convert edge map to table for export
184
185 source_ID_new = {};
186 target_ID_new = {};
187 edge_weight_new = [];
188
189 new_source_IDs = keys(new_edges);
190 edge_index = 0;
191
192 for i = 1:size(new_source_IDs, 2)
193
194     target_IDs_i = keys(new_edges(new_source_IDs{i}));
195     tmp = new_edges(new_source_IDs{i});
196
197     for j = 1:size(target_IDs_i, 2)
198
199         edge_index = edge_index + 1;
200         source_ID_new{edge_index, 1} = new_source_IDs{i};
201         target_ID_new{edge_index, 1} = target_IDs_i{j};
202         edge_weight_new(edge_index, 1) = tmp(target_IDs_i{j});
203
204     end
205
206 end
207
208 origin = source_ID_new;
209 destination = target_ID_new;
210 n = edge_weight_new;
211 new_edge_table = table(origin, destination, n);
212
213 writetable(new_edge_table, output_filename);
214
215
216 % OR, using the matrix implementation -
217 % note- this will cause memory issues if the matrices are large
218

```

```
219
220 G = [10, 100; 0, 1000]
221 P_O = [0.5, 0.4, 0.1; 0.5, 0.2, 0.3];
222 P_D = [0.4, 0.3, 0.3; 0.1, 0.3, 0.6];
223
224 G_star = P_O' * G * P_D
```
